# Supplementary material for: Bayesian analysis of diffusion-driven multi-type epidemic models with application to COVID-19
Source: arXiv:2211.15229 ancillary file (2025-09-01)
Supplement: Supplementary file 1 [file IndepBM_supplementary.pdf]

# Supplementary material to "Bayesian analysis of diffusion-driven multi-type epidemic models with application to COVID-19"

Lampros Bouranis*,[1], Nikolaos Demiris[1],
Konstantinos Kalogeropoulos[2], Ioannis Ntzoufras[1]

[1] *Department of Statistics, Athens University of Economics and Business, Athens, Greece*

[2] *Department of Statistics, The London School of Economics and Political Science, London, United kingdom*

* bouranis@aueb.gr

# S1 Data description

Table S1 presents the data sources and their definitions for England, Greece and Austria. Following the scheme in Figure 1 (see Section 2.2.1), the Bayesian evidence synthesis framework utilizes COVID-19 healthcare surveillance data, the age distribution of the population of a given country and estimated contact matrices, which are publicly available.

# S2 Bayesian inference and computational considerations

Healthcare surveillance data and expert knowledge were combined through a Bayesian hierarchical model using evidence synthesis for each country. The Bayesian paradigm allows to fully propagate the uncertainty about the unknown parameters by assigning a probability distribution to those parameters of interest that are therefore regarded as random variables, i.e a prior $\pi(\theta^{MBM})$ is first assigned on the parameter vector $\theta^{MBM}$.

The log-posterior distribution of the unknown quantities is $\log \pi(\theta \mid y) \propto \ell^{Deaths}(y \mid \theta) + \log \pi(\theta)$ for a given model. As usual in Bayesian high-dimensional models, the posterior distribution is not available in closed form, so we used Markov chain Monte Carlo (MCMC) for Bayesian parameter inference and model fitting. Thus, MCMC implementation details and modeling design choices are discussed below.

## S2.1 Computational considerations

The age-stratified transmission dynamics depend, among others, on the initial conditions of the system of non-linear ODEs. The date of simulation start $t_0$ is set on the day before the date of the first data point $t_1$ (Table S2). At $t_0$, most individuals are assumed to be susceptible and are distributed across age groups according to the population age distribution $\mathbb{N}_\alpha$ for $\alpha \in \{1,\ldots,A\}$.

The number of people in the exposed compartments at $t_0$ is controlled by a parameter $\rho$ (Table S2), and also distributed according to $\mathbb{N}_\alpha$ for $\alpha \in \{1,\ldots,A\}$. Other compartments are set to zero (Hauser et al., 2020).

The posterior distributions were estimated by sampling 500 iterations after 500 iterations for warm-up in six independent chains in the probabilistic programming language Stan (Carpenter et al., 2017) via a dynamic Hamiltonian Monte Carlo algorithm (Betancourt, 2018). In an attempt to improve convergence of the MCMC algorithm, the initial parameters for the sampler were set to the maximum a-posteriori estimates of the Bayesian model, which are cheap to compute. Convergence was assessed visually with traceplots, and numerically with the potential scale reduction statistic (Gelman and Rubin, 1992) and the effective sample size. The presence of divergent transitions was also checked. No issues with mixing and convergence were detected, in all settings. Uncertainty is expressed through 50% credible intervals (CrI) derived from the 25% and 75% quantiles and through 95% credible intervals (CrI) derived from the 2.5% and 97.5% quantiles. Computations for this work were carried out with the statistical environment R (R Core Team, 2022) on multiple desktop computers with an Intel ®Core$^{\text{TM}}$ i7-4790U CPU (3.60GHz) and 24GB RAM each, at the Laboratory of Statistical Methodology and at the Computational and Bayesian Statistics Laboratory of Athens University of Economics and Business.

## S2.2 Prior distributions

The unknown quantities that need to be inferred are $\theta^{SBM} = (x_0, x_{1:T}, C_{\alpha,\alpha'}, \sigma_x, \rho, \phi)$ and $\theta^{MBM} = (x_0^{\alpha\alpha}, x_{1:T}^{\alpha\alpha}, C_{\alpha,\alpha'}, \sigma_{x,\alpha}, \rho, \phi)$ for $\alpha \in \{1,\ldots,A\}$ for $(\alpha,\alpha') \in \{1,\ldots,A\}^2$, under the SBM and MBM model, respectively. The prior distributions placed in the parameters $\theta^{SBM}$ and $\theta^{MBM}$ are listed in Table S2. The model parameters under estimation are presented in the upper part of the table. The model also includes natural history parameters which are considered as fixed constants with their values specified from previous studies (bottom part of the table). A brief justification of the chosen prior/value is given, wherever possible.

A prior distribution was imposed on the contact matrix $C$. This was necessary in order to account for the uncertainty over the contact structure while estimating disease transmission. To achieve this, we implemented a non-centered parameterization (Papaspiliopoulos et al., 2007) which takes advantage of properties of symmetric matrices. Under this perspective, let us consider a positive-definite symmetric matrix $M$ given by

$$M = \begin{bmatrix} \mathbb{N}_1 & \ldots & 0 \\ \vdots & \ddots & \vdots \\ 0 & \ldots & \mathbb{N}_A \end{bmatrix} \cdot \begin{bmatrix} C_{1,1} & \ldots & C_{1,A} \\ \vdots & \ddots & \vdots \\ C_{A,1} & \ldots & C_{A,A} \end{bmatrix},$$

which is Cholesky factored to a lower triangular matrix $L$ such that $LL^T = M$. The Cholesky factor $L$ requires $\frac{A(A+1)}{2}$ unconstrained parameters. The elements of the lower-triangular random matrix $\tilde{L}$ are drawn from $\frac{A(A+1)}{2}$ i.i.d. standard Normal distributions. Then, a positive-definite symmetric matrix $M^{syth}$ is constructed, informed by the country-specific synthetic contact matrix $C^{syth}$ with values taken from Prem et al. (2021),

$$M^{syth} = \begin{bmatrix} \mathbb{N}_1 & \ldots & 0 \\ \vdots & \ddots & \vdots \\ 0 & \ldots & \mathbb{N}_A \end{bmatrix} \cdot \begin{bmatrix} C^{syth}_{1,1} & \ldots & C^{syth}_{1,A} \\ \vdots & \ddots & \vdots \\ C^{syth}_{A,1} & \ldots & C^{syth}_{A,A} \end{bmatrix},$$

which is Cholesky factored to a lower triangular matrix $L^{syth}$ such that $L^{syth}(L^{syth})^T = M^{syth}$. The elements of $L$ are assigned an informative Normal prior distribution $L_{i,j} \sim \mathrm{N}(L^{syth}_{i,j}, (0.05 \cdot L^{syth}_{i,j})^2)$, respectively $L_{i,j} = L^{syth}_{i,j} + (0.05 \cdot L^{syth}_{i,j}) \cdot \tilde{L}_{i,j}$, $(i,j) \in \{1,\ldots,A\}^2$. The random contact matrix $C$ is, then, given by

$$C = \begin{bmatrix} \mathbb{N}_1 & \ldots & 0 \\ \vdots & \ddots & \vdots \\ 0 & \ldots & \mathbb{N}_A \end{bmatrix}^{-1} \cdot LL^T. \tag{S.1}$$

Finally, we note that the observation model was fine-tuned to the Austrian age-stratified mortality counts under the MBM transmission model; the results presented below are based on the over-dispersed count model

$$y_{t,\alpha} \mid \theta^{MBM} \sim \mathrm{NegBin}\,(d_{t,\alpha}, \phi), \tag{S.2}$$

where $\mathbb{E}[y_{t,\alpha}] = d_{t,\alpha}$ and $\mathbb{V}[y_{t,\alpha}] = d_{t,\alpha} + \frac{d_{t,\alpha}}{\phi}$, assuming $\phi \sim$ Half-Normal$(0,5)$ and informative priors for the age-stratified volatility paramters $\sigma_{x,\alpha} \sim \mathrm{Gamma}(1,1), \alpha \in \{1,\ldots,A\}$.

# S3 Model fitting and model determination

We performed a quantitative assessment of the fit of the SBM and MBM transmission models to the data by comparing the Deviance information criterion (DIC, Spiegelhalter et al. 2002) and the approximate Pareto smoothed importance sampling leave-one-out cross-validation information criterion (CVIC, Vehtari et al. 2017). The effective number of parameters was estimated under the respective criterion. The model that gave the lowest DIC/CVIC would be selected as the most appropriate, accounting for the approximate standard error of the estimate (Table S3).

Cross-validation and information criteria are two approaches to estimating out-of-sample predictive accuracy using within-sample fits. Both the DIC and CVIC are cheap approximations to the computationally intensive cross-validation process (whether calculated directly by refitting each model to several different data subsets) of the model proposed in this work.

The latent sample paths of the diffusions are infinite-dimensional objects. We adopted the data augmentation framework of Dureau et al. (2013) as a means to infer the latent sample path(s). For the study period of $K = 30$ weeks, we observe that the estimated number of parameters for each model is less than $K$ for both countries. For Greece both criteria suggest non-identifiability and cannot differentiate between the two models (Table S3). For Austria, model determination is also inconclusive.

Posterior predictive checking involves comparing the observed data to simulated samples generated from the posterior predictive distribution of a given model. We proceeded with graphical checks where the observed age-stratified mortality counts and the observed mortality counts summed over age groups were compared to those for simulated samples.

Any systematic differences between simulated samples and observed data indicate potential shortcomings of the model. If the given model fits the data, then replicated data generated under the model should look similar to the observed data. If the observed data is not plausible under the posterior predictive distribution, this could indicate that the model is not a good fit for the data.

For Greece, both models appear to fit the data (Figures S1 and S2) and uncertainty in the generated data appears to decrease with age (more informed contexts). We can reach the same conclusions for the case of Austria (Figures S3 and S4). In light of these findings, the qualitative

comparison of the two models discussed in Section 3.2 with respect to their ability to infer the age-stratified dynamic transmission rates provides the last piece in the puzzle of model fitting and model determination.

# S4 Age-stratified transmission rate

The analysis of Austrian age-stratified mortality counts reveals the difficulty of the SBM model to break down the age-stratified transmission rate $m^{\mathrm{SBM}}_{\alpha,\alpha'}(t)$ into its biological and social components (Figure S5, Panels A-B).

Given that the SBM model forces the age-stratified transmissibilities to be expressed by an overall effective contact rate for the population, we observe a shift between the prior and posterior contact rates, reflecting the effect that interventions had in human behaviour during the study period (Figure S5, panel B). The age-stratified transmission rate trajectories (Figure S5, panel C) only differ in terms of magnitude at the time-points of the observations.

The posterior age-stratified transmission rate trajectories under the MBM model (Figure S6, panel C) enable the assessment of interventions (Table S4) in transmission. The mandatory use of masks in all public spaces did not appear to reduce virus transmission until 3 weeks later, in the beginning of October 2020. Restrictions on private gatherings helped reduce transmission in both age groups in October 2020; interventions to limit all in- door/outdoor mass/public gatherings, as well as the implementation of a lockdown, kept virus transmission to low levels until the beginning of December 2020. While relaxation of lockdown measures kept transmission of the $\{65+\}$ age group to a low level, it did not stop an increase in transmission for the $\{< 65\}$ age group. Since the beginning of January 2021, there was an increasing trend in transmission of the $\{< 65\}$ age group, while transmission for the elders remained low, albeit with some fluctuations until the end of the study period.

# S5 Estimated age-stratified latent infections

Denote the estimated new daily infections by $\Delta^{\mathrm{infec}}_{t} = \sum_{\alpha=1}^{A} \Delta^{\mathrm{infec}}_{t,\alpha}$. The posterior distributions $\pi(\Delta^{\mathrm{infec}}_{t,\alpha} \mid y_{t,\alpha}), \alpha \in \{0-39, 40-64, 65+\}$, and $\pi(\Delta^{\mathrm{infec}}_{t} \mid y)$ for Greece are shown in Figure S7. The posterior distributions $\pi(\Delta^{\mathrm{infec}}_{t,\alpha} \mid y_{t,\alpha}), \alpha \in \{< 65, 65+\}$, and $\pi(\Delta^{\mathrm{infec}}_{t} \mid y)$ for Austria are shown in Figure S8 and S9, respectively.

Greater uncertainty is observed in the posterior estimates $\pi(\Delta^{\mathrm{infec}}_{t,\alpha} \mid y_{t,\alpha})$ and $\pi(\Delta^{\mathrm{infec}}_{t} \mid y)$ nearly the end of the study period: by construction of the observation model, the age-stratified mortality counts enable a more accurate estimation of the age-stratified infections in the past 3 weeks (Figures S7-S9). Additionally, the low mortality counts in the youngest age group result in estimated age-stratified infections with larger uncertainty, which is reflected in the wider credible intervals of the model estimates (Figure S7, Panel A).

For the case of Greece, the higher age-stratified mortality counts in the beginning of December 2020 yielded an increased number of estimated age-stratified infections around 3 weeks earlier. During this period which corresponds to the second wave of the SARS-Cov-2 pandemic in Greece, the estimated age-stratified daily new infections are significantly higher than the laboratory-confirmed infections. Irrespectively of the age group, the posterior estimates and the respective credible intervals are skewed to some degree compared to the reported infections, owing to reporting delays, virus transmission via asymptomatic individuals and a change in the infection-to-death distribution in contrast to the parametric assumptions that have been made (i.e. it is assumed to be the same across age groups and constant during the study period).

For the case of Austria (Figures S8-S9), the parametric assumptions made for the infection-to-death distribution in the observation model appear to be more appropriate, as the posterior age-stratified estimates and the respective credible intervals do not appear to be skewed compared to the reported age-stratified infections. The reporting rate for the elder age group appears to be higher that the reporting rate for the younger age group most of the time during the study period.

# S6 Effective reproduction number

A method for tracking the progress of an outbreak is measuring changes in the effective reproduction number over time, $R_t^{eff}$, $t = 1, \ldots, T$, which was calculated using next generation matrix methods (Diekmann et al., 2010; Davies et al., 2020; Knock et al., 2021). $R_t^{eff}$ is defined as the average number of secondary infections generated by a case infected at day $t$, accounting for the finite population size and potential immunity in the population.

The next generation matrix was calculated for $(\alpha, \alpha') \in \{1, \ldots, A\}^2$ under the MBM transmission model as

$$\text{NGM}_{\alpha,\alpha'}(t) = m_{\alpha,\alpha'}^{\text{MBM}}(t) d_I \frac{S_\alpha(t)}{\mathbb{N}_{\alpha'}}, \tag{S.3}$$

where $\mathbb{N}_{\alpha'}$ is the population of age group $\alpha'$ and $R_t^{eff}$ is the absolute value of the dominant eigenvalue of $\text{NGM}(t)$.

By construction of the proposed model in this work, the effective reproduction number is estimated from the daily age-stratified mortality counts, accounting for variations in transmissibility that are not obvious from reported infection counts. Additionally, the NGM is a non-linear functional of the central model parameters. While estimation of the uncertainty over the effective reproduction number is itself a challenging problem (Gostic et al., 2020), it is propagated naturally via MCMC in this work. The $R_t^{eff}$ method and its changes over time can quantify the impact of public health interventions. When $R_t^{eff} < 1$, the SARS-Cov-2 pandemic is self-limiting and said to be under control due to containment strategies.

The posterior distributions $\pi(R_t^{eff} \mid y)$ for Greece and Austria are shown in Figures S10 and S11, respectively. In Greece, the nationwide lockdown that was imposed in early November 2020 sustained a low spread of the SARS-Cov-2 virus until the end of January 2021, reflected in the estimated effective reproduction number which remained below 1. The establishment of more transmissible SARS-Cov-2 variants and relaxation of the imposed measures during the Christmas holidays led to a gradual increase in $R_t^{eff}$ in Greece until the first week of February 2021.

In Austria, the mandatory use of masks in all public spaces that was imposed in mid-September 2020 was successful in intercepting virus transmission around 3 weeks later, with the estimated effective reproduction number gradually decreasing from its highest point during the study period to values below 1 in mid-October 2020. The restrictions on gatherings and the national lockdown were successful in restraining the transmission of the virus.

# S7 Age-stratified reporting ratio

Let $\hat{\Delta}_{t-L,\alpha}^{\text{infec,pop}}, \alpha \in \{1, \ldots, A\}$ denote the age-stratified posterior median of the number of new infected individuals in the population at time $t - L$, which allows for a reporting delay of $L$ days between infection and report; the number of new age-stratified laboratory-confirmed infections

which are reported at time $t$ is denoted by $\Delta_{t,\alpha}^{\text{infec,rep}}$. The estimated age-stratified daily reporting ratio for $\alpha \in \{1,\ldots,A\}$ is expressed by

$$\hat{r}_{t,\alpha} = \frac{\Delta_{t,\alpha}^{\text{infec,rep}}}{\hat{\Delta}_{t-L,\alpha}^{\text{infec,pop}}}.$$

We considered a time delay between infection and report ($L$) equal to 6 days; a time-varying spline-based smoother was applied to $\hat{r}_{t,\alpha}$ via generalized additive model smoothing (Wood et al., 2016).

Our analysis indicates that during periods of high transmission a large proportion of under-reported infections is present (Figures S12 and S13), resulting in low age-stratified reporting ratios. In Greece, the highest reporting ratios during the study period are observed in October 2020; a higher estimate is reported for the youngest age group which appears 2-3 weeks later compared to the other age groups, reflecting the skewness that is visible in the estimated age-stratified infections compared to the reported age-stratified infections (Figure S7). For the elders, the estimated reporting ratio appears to remain at about 50% from early December 2020 until the end of the study period, while the respective estimates for the other age groups demonstrate fluctuations.

In Austria, the elders have an estimated reporting ratio which deviates around 40-60% for the majority of the study period (Figure S13), while for the $\{< 65\}$ age group is estimated reporting ratio drops below 40% at early November 2020, following the implementation of stricter virus containment strategies.

# References


Betancourt, M. (2018). A conceptual introduction to Hamiltonian Monte Carlo. `https://arxiv.org/abs/1701.02434`.

Birrell, P., Blake, J., van Leeuwen, E., Gent, N., and De Angelis, D. (2021). Real-time nowcasting and forecasting of COVID-19 dynamics in England: the first wave. *Phil. Trans. R. Soc. B*, 376:20200279.

Caporali, A., Garcia, J., Couppie, E., Poniakina, S., M., B., Bonnet, F., Camarda, C., Cambois, E., Hourani, I., Korotkova, D., Mesle, F., Penina, O., Robine, J., Sauerberg, M., and Catalina Torres, C. (2022). The demography of covid-19 deaths database, a gateway to well-documented international data. *Scientific Data*, 9:1–9.

Carpenter, B., Gelman, A., Hoffman, M., Lee, D., Goodrich, B., Betancourt, M., Brubaker, M., Guo, J., Li, P., and Riddell, A. (2017). Stan: A probabilistic programming language. *Journal of statistical software*, 76(1):1–32.

Davies, N., Klepac, P., Liu, Y., Prem, K., Jit, M., CMMID COVID-19 working group, and Eggo, R. (2020). Age-dependent effects in the transmission and control of COVID-19 epidemics. *Nat Med*, 26:1205–1211.

Diekmann, O., Heesterbeek, J., and Roberts, M. (2010). The construction of next-generation matrices for compartmental epidemic models. *J. R. Soc. Interface*, 7:873–885.

Dureau, J., Kalogeropoulos, K., and Baguelin, M. (2013). Capturing the time-varying drivers of an epidemic using stochastic dynamical systems. *Biostatistics*, 14(3):541–555.

Gelman, A. and Rubin, D. (1992). Inference from iterative simulation using multiple sequences. *Statistical Science*, 7(4):457–472.

Gostic, K., McGough, L., Baskerville, E., Abbott, S., Joshi, K., Tedijanto, C., Kahn, R., Niehus, R., Hay, J., De Salazar, P., Hellewell, J., Meakin, S., Munday, J., Bosse, N., Sherrat, K., Thompson, R., White, L., Huisman, J., Scire, J., Bonhoeffer, S., Stadler, T., Wallinga, J., Funk, S., Lipsitch, M., and Cobey, S. (2020). Practical considerations for measuring the effective reproductive number, Rt. *PLOS Computational Biology*, 16(12):1–21.

Hauser, A., Counotte, M., Margossian, C., Konstantinoudis, G., Low, N., Althaus, C., and Riou, J. (2020). Estimation of SARS-CoV-2 mortality during the early stages of an epidemic: A modeling study in Hubei, China, and six regions in Europe. *PLOS Medicine*, 17(7):1–17.

Knock, E., Whittles, L., Lees, J., Perez-Guzman, P., Verity, R., FitzJohn, R., Gaythorpe, K., Imai, N., Hinsley, W., Okell, L., Rosello, A., Kantas, N., Walters, C., Bhatia, S., Watson, O., Whittaker, C., Cattarino, L., Boonyasiri, A., Djaafara, B., Fraser, K., Fu, H., Wang, H., Xi, X., Donnelly, C., Jauneikaite, E., Laydon, D., White, P., Ghani, A., Ferguson, N., Cori, A., and Baguelin, M. (2021). Key epidemiological drivers and impact of interventions in the 2020 SARS-CoV-2 epidemic in England. *Science Translational Medicine*, 13(602):eabg4262.

Liu, T., Hu, J.and Kang, M., Lin, L., Zhong, H., Xiao, J., He, G., Song, T., Huang, Q., Rong, Z., Deng, A., Zeng, W., Tan, X., Zeng, S., Zhu, Z., Li, J., Wan, D., Lu, J., Deng, H., and Ma, W. (2020). Transmission dynamics of 2019 novel coronavirus (2019-nCoV). *The Lancet*.

National Health Service England (2022). COVID-19 Daily Deaths. `https://www.england.nhs.uk/statistics/statistical-work-areas/covid-19-daily-deaths/`.

Office for National Statistics (2022). Population and migration. `https://www.ons.gov.uk/peoplepopulationandcommunity/populationandmigration/populationestimates`.

Papaspiliopoulos, O., Roberts, G., and Sköld, M. (2007). A general framework for the parametrization of hierarchical models. *Statistical Science*, 22(1):59–73.

Prem, K., Zandvoort, K., Klepac, P., Eggo, R., Davies, N., Cook, A., and Jit, M. (2021). Projecting contact matrices in 177 geographical regions: An update and comparison with empirical data for the COVID-19 era. *PLOS Computational Biology*, 17(7):1–19.

R Core Team (2022). *R: A Language and Environment for Statistical Computing*. R Foundation for Statistical Computing, Vienna, Austria.

Sandbird (2022). Daily regional statistics for covid19 cases in greece. `https://github.com/Sandbird/covid19-Greece/`.

Spiegelhalter, D., Best, N., Carlin, B., and Van Der Linde, A. (2002). Bayesian measures of model complexity and fit. *Journal of the Royal Statistical Society: Series B (Statistical Methodology)*, 64(4):583–639.

UK Health Security Agency (2022). COVID-19 datasets. `https://coronavirus.data.gov.uk/details/download/`.

United Nations: Department of Economic and Social Affairs: Population Division (2020). *World population prospects*. United Nations, New York, NY.

Vehtari, A., Gelman, A., and Gabry, J. (2017). Practical Bayesian model evaluation using leave-one-out cross-validation and WAIC. *Statistics and Computing*, 27:1413–1432.

Ward, H., Atchison, C., Whitaker, M., Ainslie, K., Elliott, J., Okell, L., Redd, R., Ashby, D., Donnelly, C., Barclay, W., Darzi, A., Cooke, G., Riley, S., and Elliott, P. (2021). Sars-cov-2 antibody prevalence in england following the first peak of the pandemic. *Nat Commun*, 12:905.

Wood, S., Pya, N., and Säfken, B. (2016). Smoothing parameter and model selection for general smooth models. *Journal of the American Statistical Association*, 111(516):1548–1563.

Table S1: Data sources and definitions.

| Data type | Description | Source | Reference |
|---|---|---|---|
| Mortality | Daily number of new deaths by age group according to the date of death, tested positive for COVID-19. For England, hospital-only. For Austria: deaths in hospitals or elsewhere after testing positive on COVID-19, including those who died potentially from other cause. | NHS, England; Hellenic National Public Health Organization; Austrian Agency for Health and Food Safety | National Health Service England (2022); Sandbird (2022); Caporali et al. (2022) |
| Infections | Daily number of new infections by age group and specimen date | NHS, England; Hellenic National Public Health Organization; Austrian Agency for Health and Food Safety | UK Health Security Agency (2022); Sandbird (2022); Caporali et al. (2022) |
| Age distribution | Age distribution for a given year, broken down by 5-year age bands and gender | United Nations; Office for National Statistics, UK | United Nations: Department of Economic and Social Affairs: Population Division (2020); Office for National Statistics (2022) |
| Contact matrix | Rate of contacts between age groups | | Prem et al. (2021) |

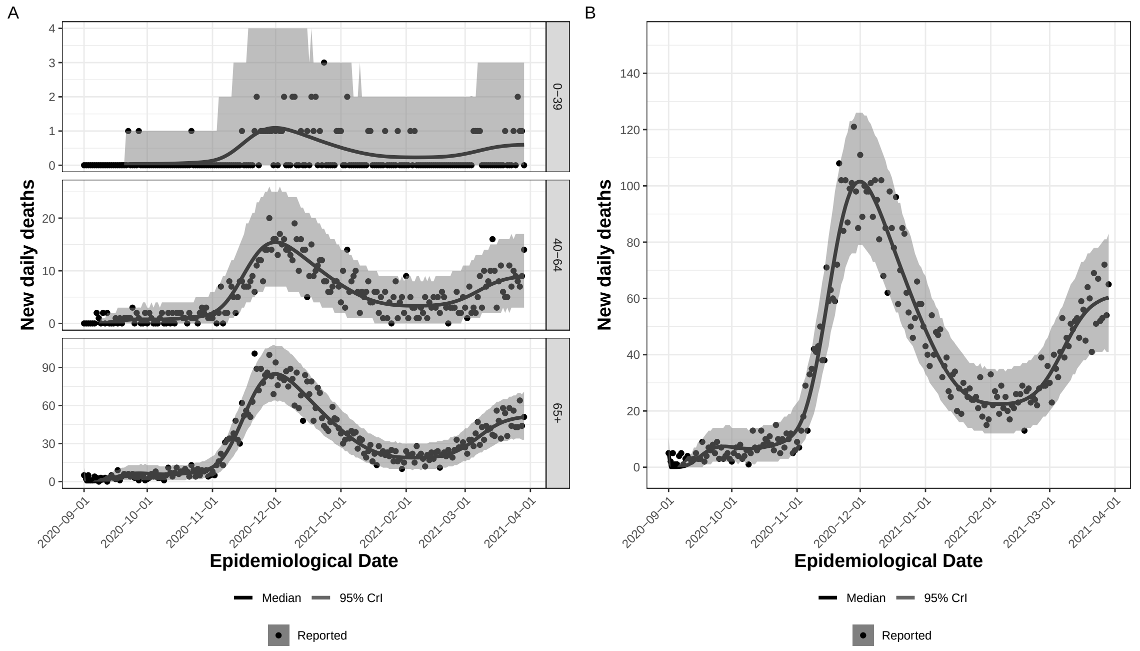


Figure S1: Greece - Goodness-of-fit under the SBM transmission model against the reported daily mortality counts. Age-stratified expected posterior mortality counts (panel A); aggregated expected posterior mortality counts (panel B). Model estimates are based on posterior medians, together with 95% credible intervals (CrIs) of draws from the posterior predictive distribution.

Table S2: Model parameters with assumed prior distributions or fixed values.

| Symbol | Description | Prior & source |
|---|---|---|
| **Transmission model parameters** | | |
| $\rho$ | Initial proportion of exposed (at time $t_0$) | Beta with $\mathbb{E}[\rho] = 0.1$, $\mathbb{V}[\rho] = 0.05 \cdot \mathbb{E}[\rho]$. Based on Hauser et al. (2020). |
| $\tilde{L}_{i,j}$ | Lower-triangular random matrix | $\tilde{L}_{i,j} \sim \text{Normal}(0,1)$, $(i,j) \in \{1,\ldots,A\}^2, i \leq j$. |
| $L_{i,j}$ | Entries of the Cholesky factor $L$ | $L_{i,j} = L^{synth}_{i,j} + (0.05 \cdot L^{synth}_{i,j}) \cdot \tilde{L}_{i,j}$, $(i,j) \in \{1,\ldots,A\}^2, i \leq j$. |
| $x_0$ | SBM model Brownian motion, at time $t_0$ | $\text{Normal}(0,5^2)$ |
| $x_1$ | SBM model Brownian motion, at time $t_1$ | $\text{Normal}(0,5^2)$ |
| $x_t$ | SBM model Brownian motion | $x_t \mid x_{t-1}, \sigma_x^2 \sim \text{Normal}(x_{t-1}, \sigma_x^2)$, $t = 2,\ldots,T$. |
| $x_0^{\alpha\alpha}$ | MBM model Brownian motion, at time $t_0$ | $\text{Normal}(0,5^2)$ |
| $x_1^{\alpha\alpha}$ | MBM model Brownian motion, at time $t_1$ | $\text{Normal}(0,5^2)$ |
| $x_t^{\alpha\alpha}$ | MBM model Brownian motion at time $t$ | $x_t^{\alpha\alpha} \mid x_{t-1}^{\alpha\alpha}, \sigma_{x,\alpha}^2 \sim \text{Normal}(x_{t-1}^{\alpha\alpha}, \sigma_{x,\alpha}^2)$, $t = 2,\ldots,T$. |
| $\sigma_x$ | Volatility of the Brownian motion in the SBM model | Half-Normal$(0,4)$. |
| $\sigma_{x,\alpha}$ | Volatility of the Brownian motion in the MBM model | Gamma$(1,1)$ for the MBM model, Austria. Otherwise, Half-Normal$(0,4)$. |
| **Observation model parameters** | | |
| $\phi$ | Negative Binomial over-dispersion | Half-Normal$(0,5)$ for the MBM model, Austria. Otherwise, Exp(0.2), based on Birrell et al. (2021). |
| **Parameters assumed known** | | |
| $\widehat{\text{IFR}}_\alpha$ | Infection-fatality rate | Informed by Ward et al. (2021). |
| $d_E$ | Mean Incubation period | 3 days. Based on Liu et al. (2020). |
| $d_I$ | Mean Infection period | 4 days. Based on Liu et al. (2020). |

Table S3: Model determination. DIC: Deviance information criterion (Spiegelhalter et al., 2002); $\hat{p}_{DIC}$: estimated effective number of parameters using the DIC; CVIC: Pareto smoothed importance sampling leave-one-out cross-validation information criterion and accompanying standard error (Vehtari et al., 2017) ; $\hat{p}_{CVIC}$: estimated effective number of parameters using CVIC and accompanying standard error.

| Country | Model | DIC | $\hat{p}_{DIC}$ | CVIC (se) | $\hat{p}_{CVIC}$ (se) |
|---|---|---|---|---|---|
| Greece | SBM | 2506.8 | 16.3 | 2507.4 (56.0) | 15.9 (1.2) |
| | MBM | 2506.6 | 26.4 | 2506.2 (57.3) | 24.6 (1.6) |
| Austria | SBM | 2212.9 | 13.7 | 2210.7 (53.8) | 10.9 (0.9) |
| | MBM | 2223.9 | 20.8 | 2222.6 (73.1) | 18.5 (1.4) |

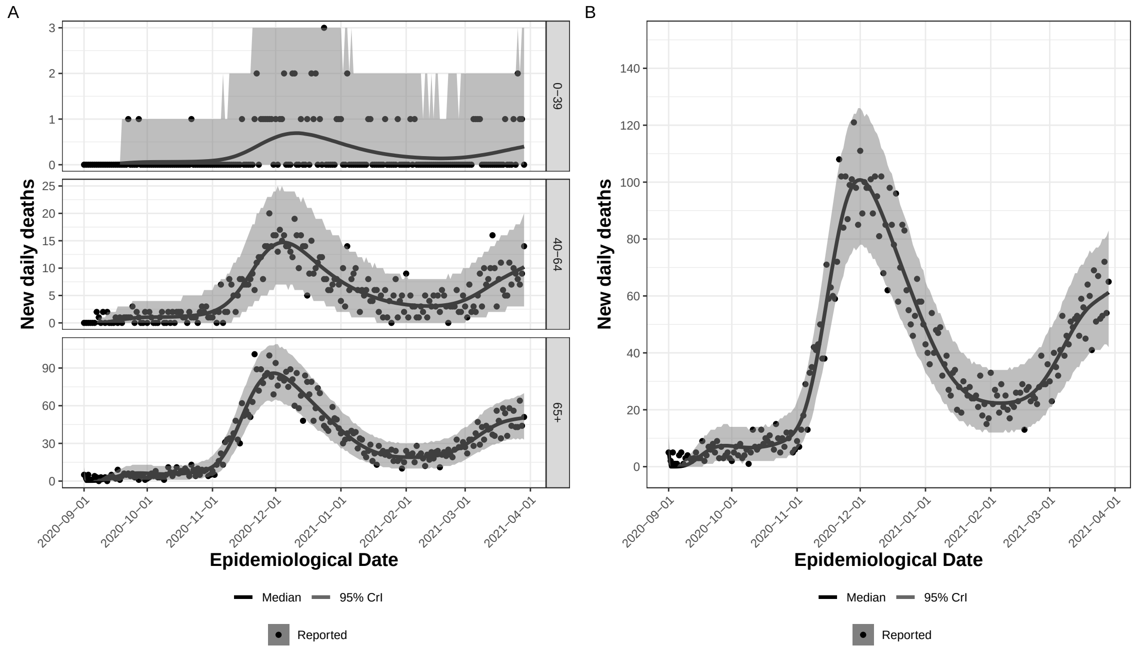


Figure S2: Greece - Goodness-of-fit under the MBM transmission model against the reported daily mortality counts. Age-stratified expected posterior mortality counts (panel A); aggregated expected posterior mortality counts (panel B). Model estimates are based on posterior medians, together with 95% credible intervals (CrIs) of draws from the posterior predictive distribution.

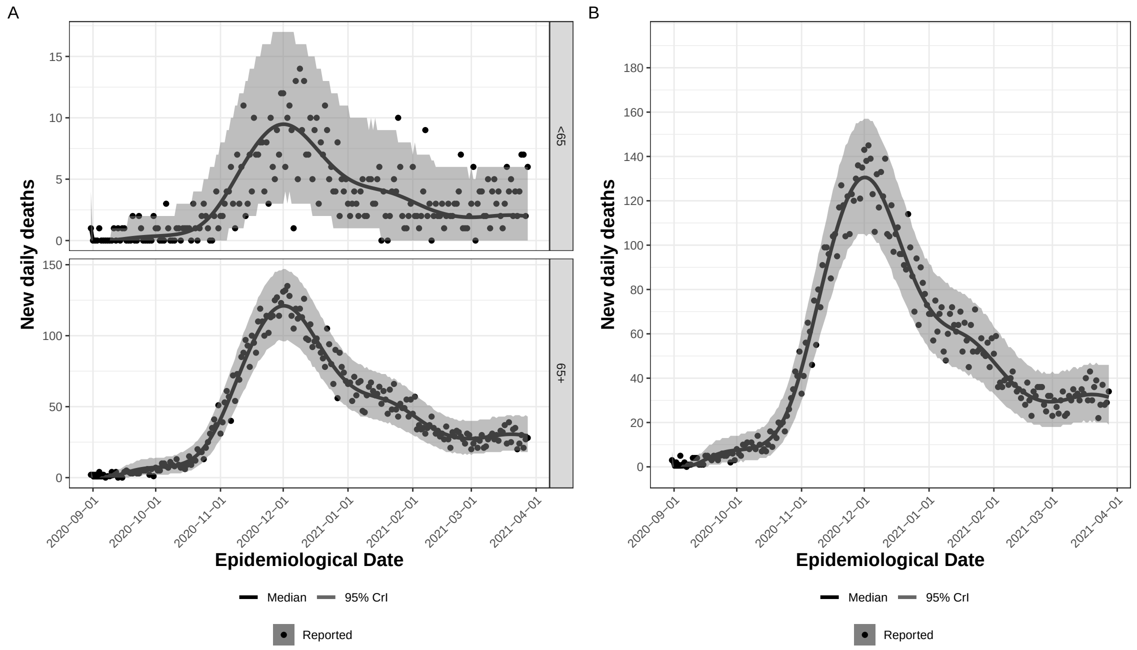


Figure S3: Austria - Goodness-of-fit under the SBM transmission model against the reported daily mortality counts. Age-stratified expected posterior mortality counts (panel A); aggregated expected posterior mortality counts (panel B). Model estimates are based on posterior medians, together with 95% credible intervals (CrIs) of draws from the posterior predictive distribution.

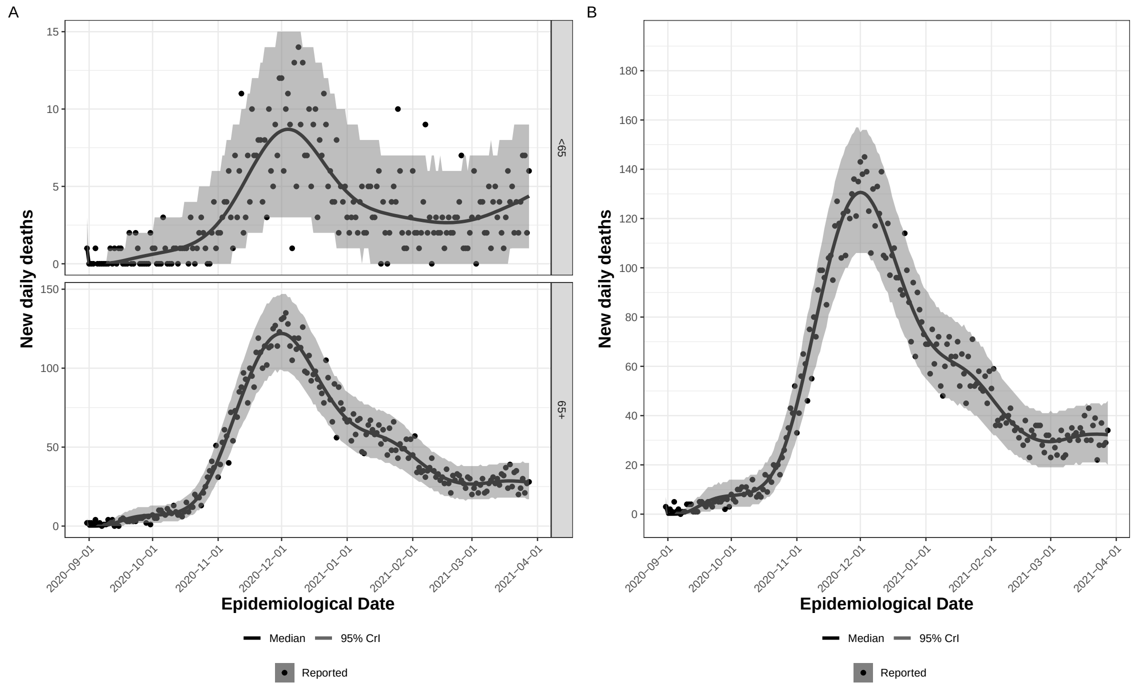


Figure S4: Austria - Goodness-of-fit under the MBM transmission model against the reported daily mortality counts. Age-stratified expected posterior mortality counts (panel A); aggregated expected posterior mortality counts (panel B). Model estimates are based on posterior medians, together with 95% credible intervals (CrIs) of draws from the posterior predictive distribution.

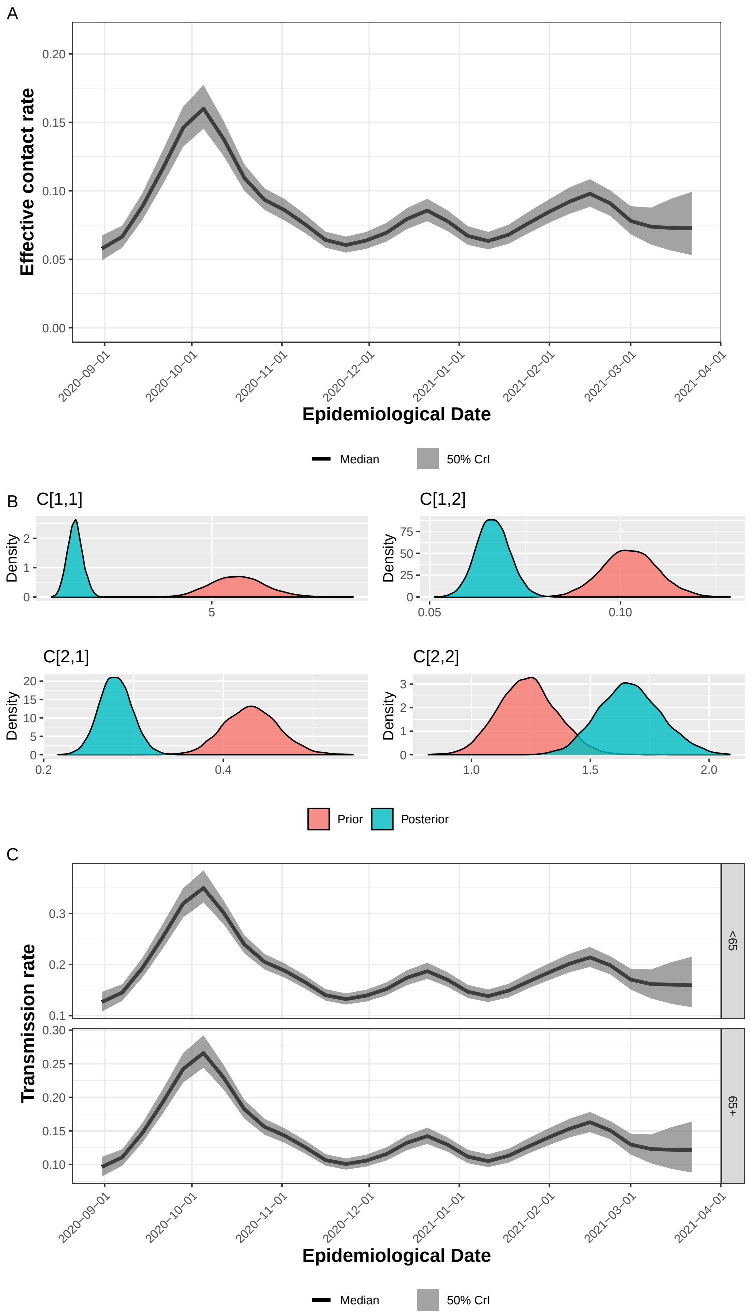


Figure S5: Austria - Components of the age-stratified transmission dynamics under the SBM transmission model. Estimated posterior trajectory (50% credible interval, CrI) of the transmissibility of SARS-CoV-2 (panel A); prior and posterior distributions of each element of the contact matrix (panel B); estimated posterior trajectory (50% credible interval, CrI) of the age-stratified transmission rate (panel C).

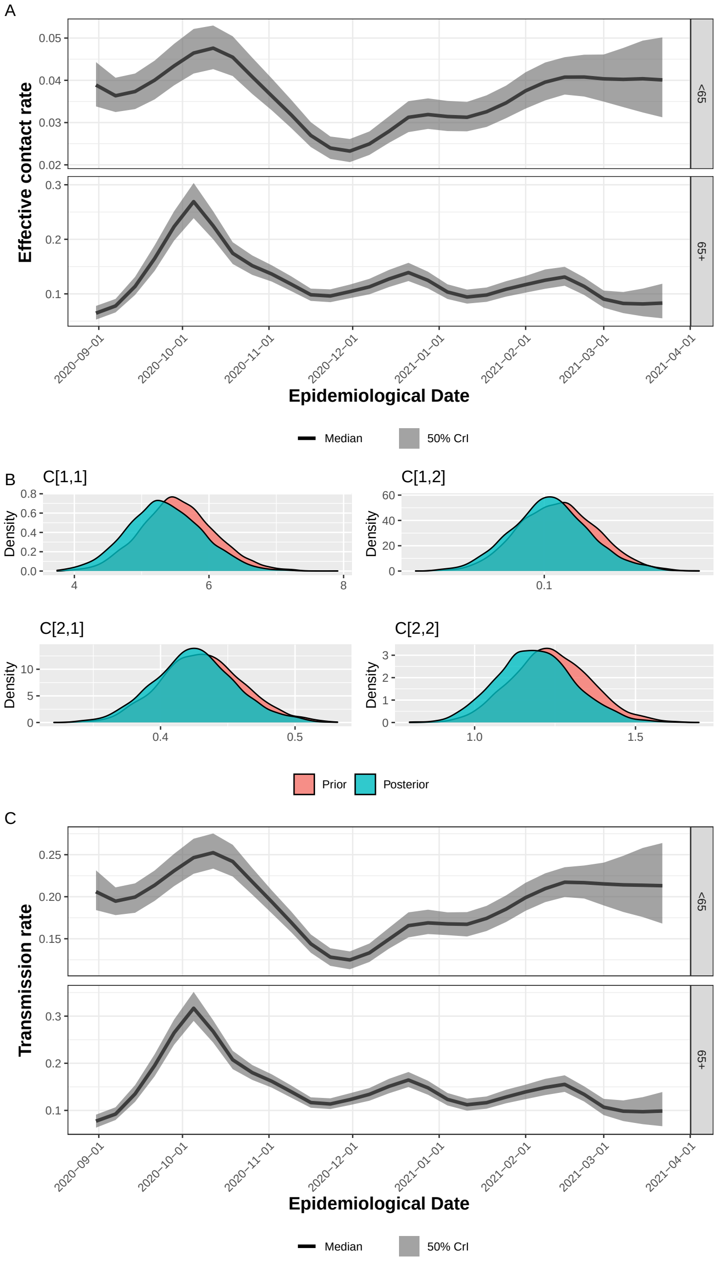


Figure S6: Austria - Components of the age-stratified transmission dynamics under the MBM transmission model. Estimated posterior trajectory (50% credible interval, CrI) of the transmissibility of SARS-CoV-2 (panel A); prior and posterior distributions of each element of the contact matrix (panel B); estimated posterior trajectory (50% credible interval, CrI) of the age-stratified transmission rate (panel C).

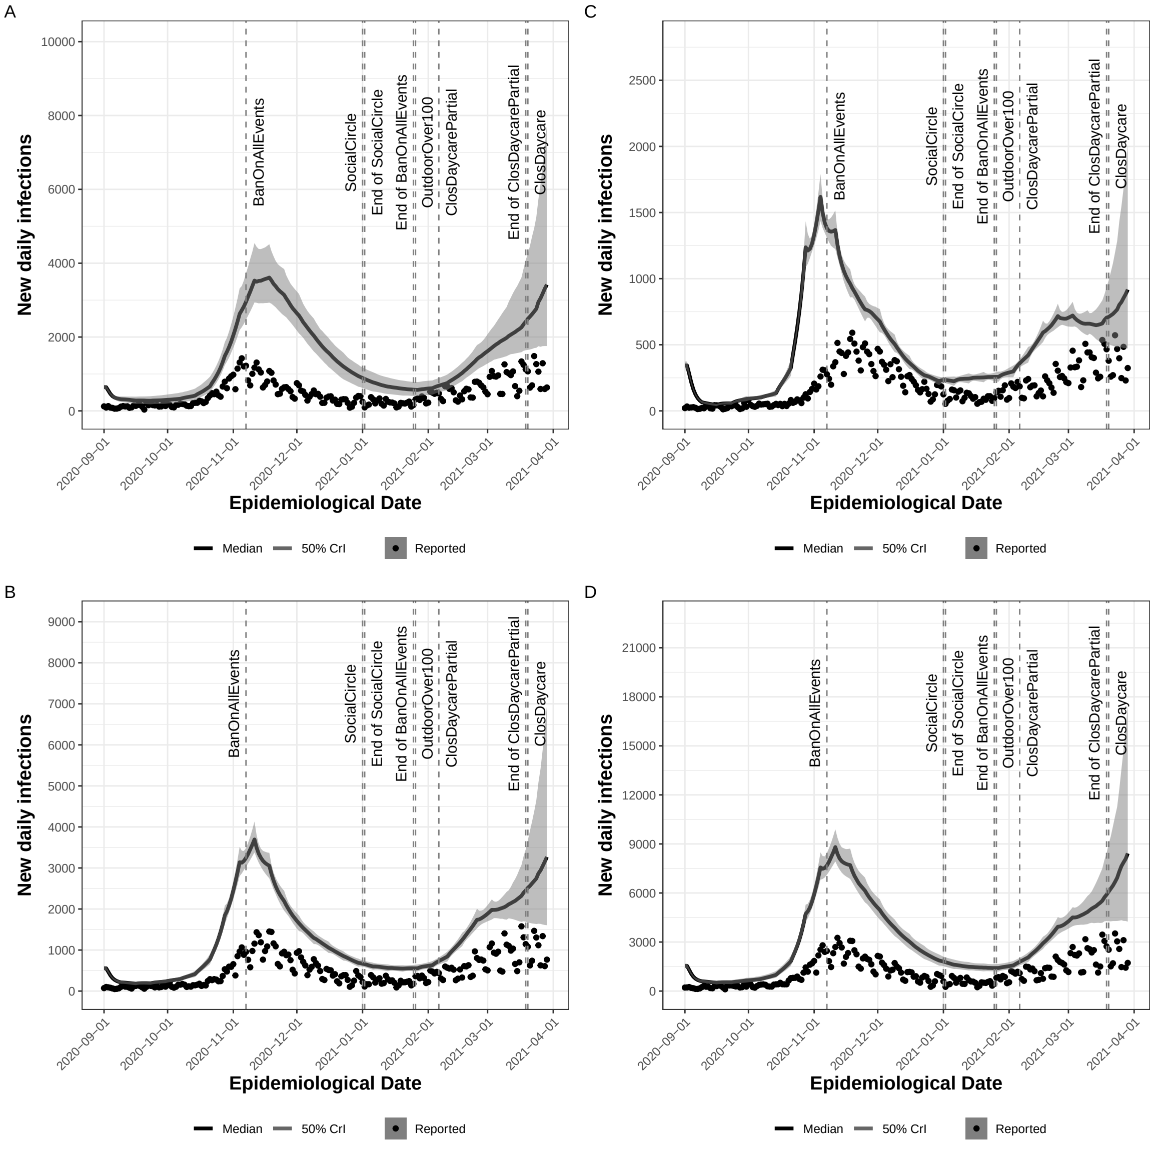


Figure S7: Greece - Estimated infections under the MBM transmission model against the laboratory-confirmed COVID-19 infections. Age group "0-39" (panel A); Age group "40-64" (panel B); Age group "65+" (panel C); aggregated infections (panel D). Model estimates are based on posterior medians, together with 50% credible intervals (CrIs).

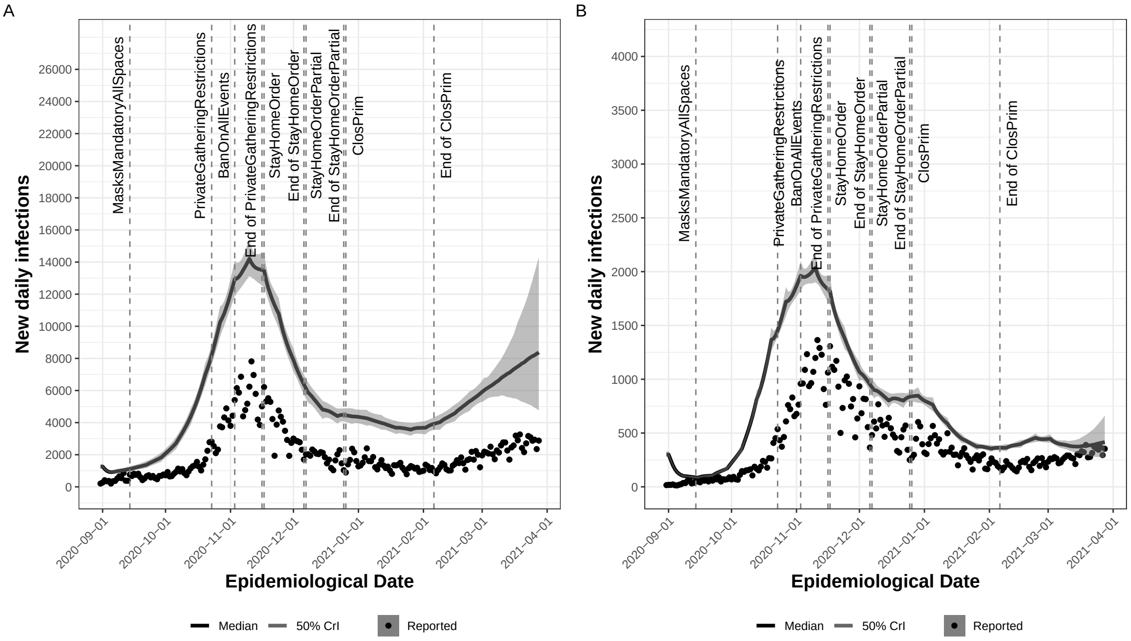


Figure S8: Austria - Estimated age-stratified infections under the MBM transmission model against the laboratory-confirmed COVID-19 infections. Age group "< 65" (panel A); Age group "65+" (panel B). Model estimates are based on posterior medians, together with 50% credible intervals (CrIs).

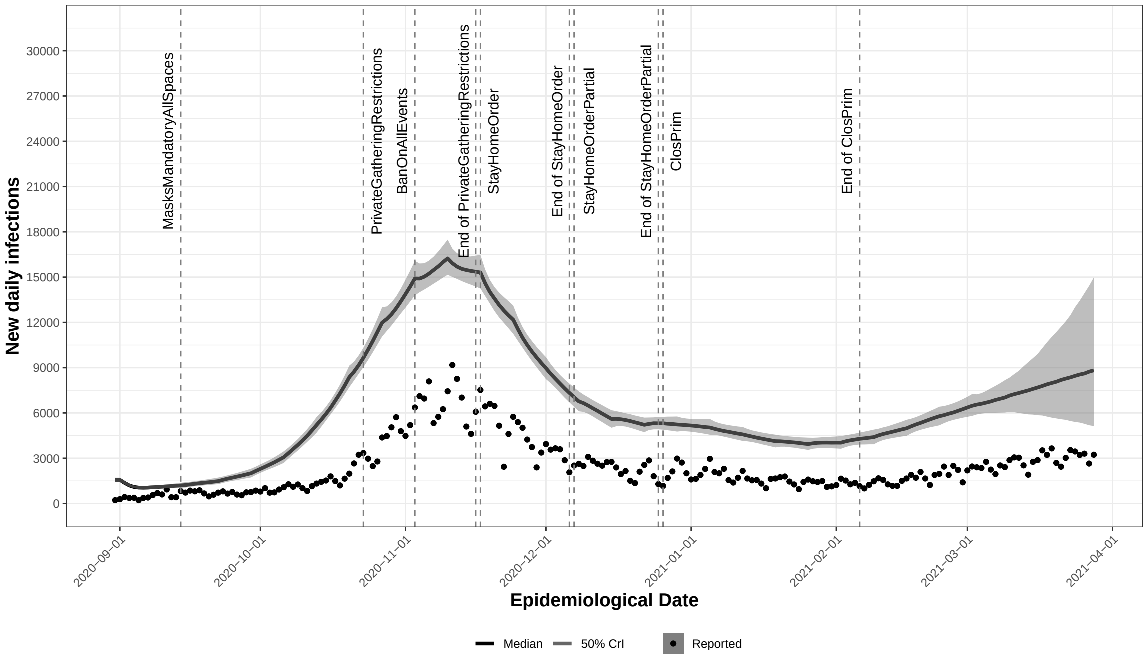


Figure S9: Austria - Aggregated expected posterior infection counts under the MBM transmission model against the laboratory-confirmed COVID-19 infections. Model estimates are based on posterior medians, together with 50% credible intervals (CrIs).

Table S4: European Centre for Disease Prevention and Control - Non-pharmaceutical interventions based on information available from official public sources.

| Country | Intervention | Definition | Start date | End date |
|---|---|---|---|---|
| Greece | BanOnAllEvents | Interventions are in place to limit all indoor/outdoor mass/public gatherings | 2020-11-07 | 2021-01-25 |
| | SocialCircle | Social circle/bubble to limit social contacts e.g. to limited number of households | 2021-01-01 | 2021-01-02 |
| | OutdoorOver100 | Interventions are in place to limit outdoor mass/public gatherings of over 100 participants | 2021-01-26 | 2021-05-20 |
| | ClosDaycarePartial | Closure of educational institutions: daycare or nursery – partially relaxed measure | 2021-02-06 | 2021-03-19 |
| | ClosDaycare | Closure of educational institutions: daycare or nursery | 2021-03-20 | 2021-05-20 |
| Austria | MasksMandatoryAllSpaces | Protective mask use in all public spaces on mandatory basis (enforced by law) | 2020-09-14 | 2021-06-09 |
| | PrivateGatheringRestrictions | Restrictions on private gatherings | 2020-10-23 | 2020-11-16 |
| | BanOnAllEvents | Interventions are in place to limit all indoor/outdoor mass/public gatherings | 2020-11-07 | 2021-01-25 |
| | StayHomeOrder | Stay-at-home orders for the general population (these are enforced and also referred to as "lockdown") | 2020-11-17 | 2020-12-06 |
| | StayHomeOrderPartial | Stay-at-home orders for the general population (these are enforced and also referred to as 'lockdown') – partially relaxed measure | 2020-12-07 | 2020-12-25 |
| | ClosPrim | Closure of educational institutions: primary schools | 2020-12-26 | 2021-02-06 |

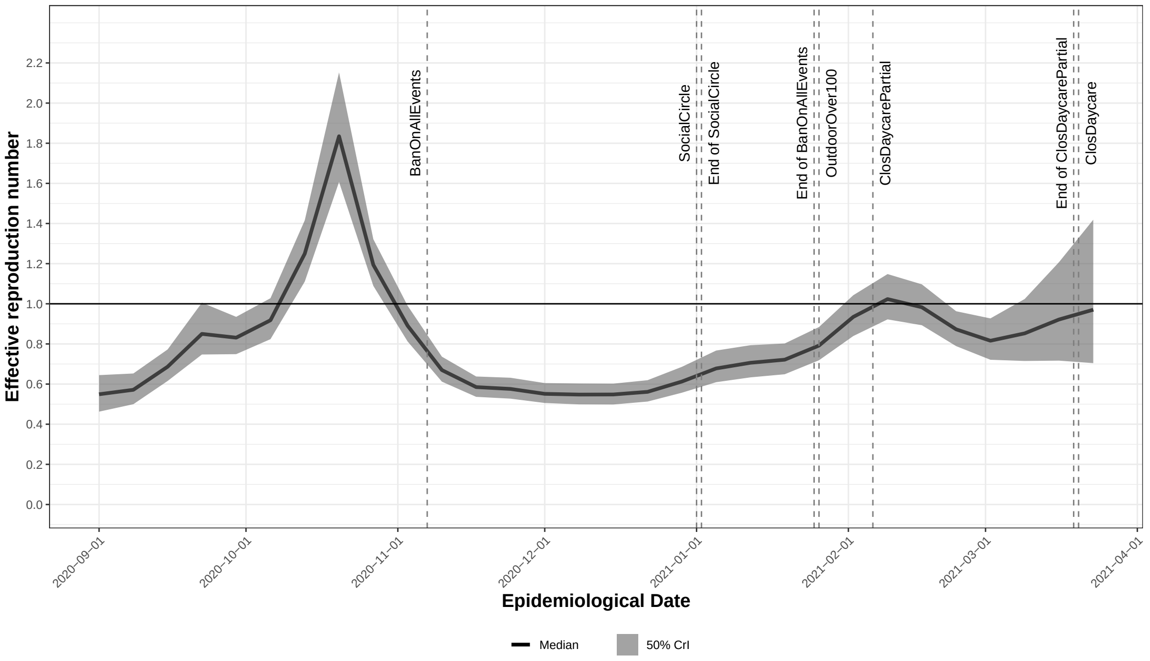


Figure S10: Greece - Posterior median (50% credible interval) effective reproduction number under the MBM transmission model.

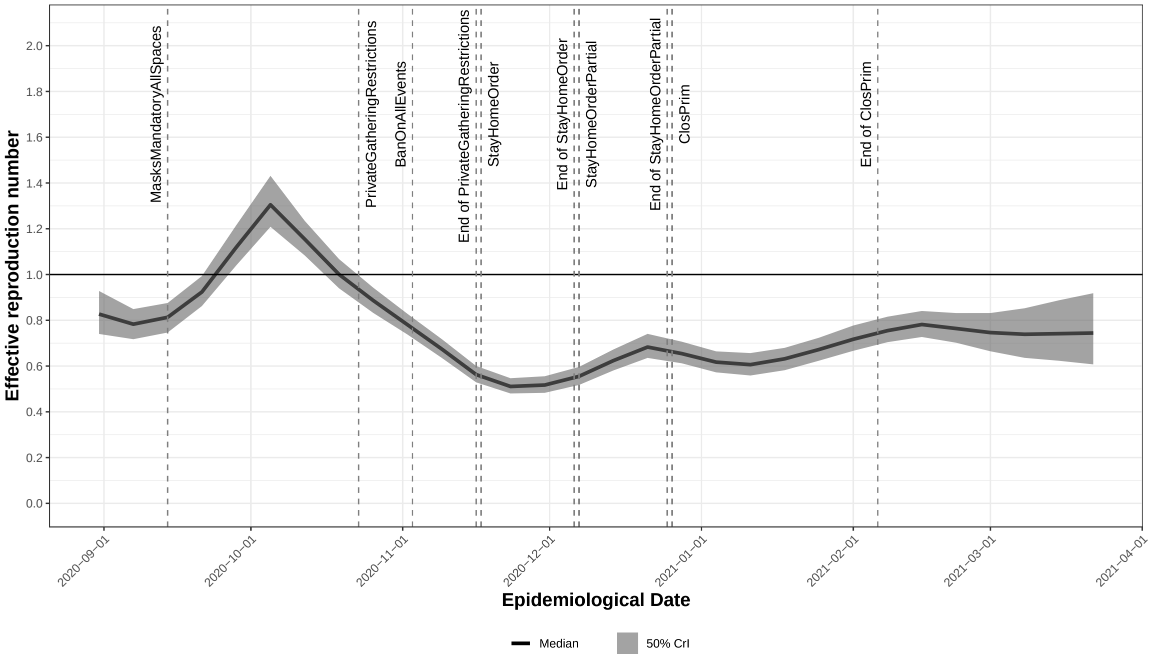


Figure S11: Austria - Posterior median (50% credible interval) effective reproduction number under the MBM transmission model.

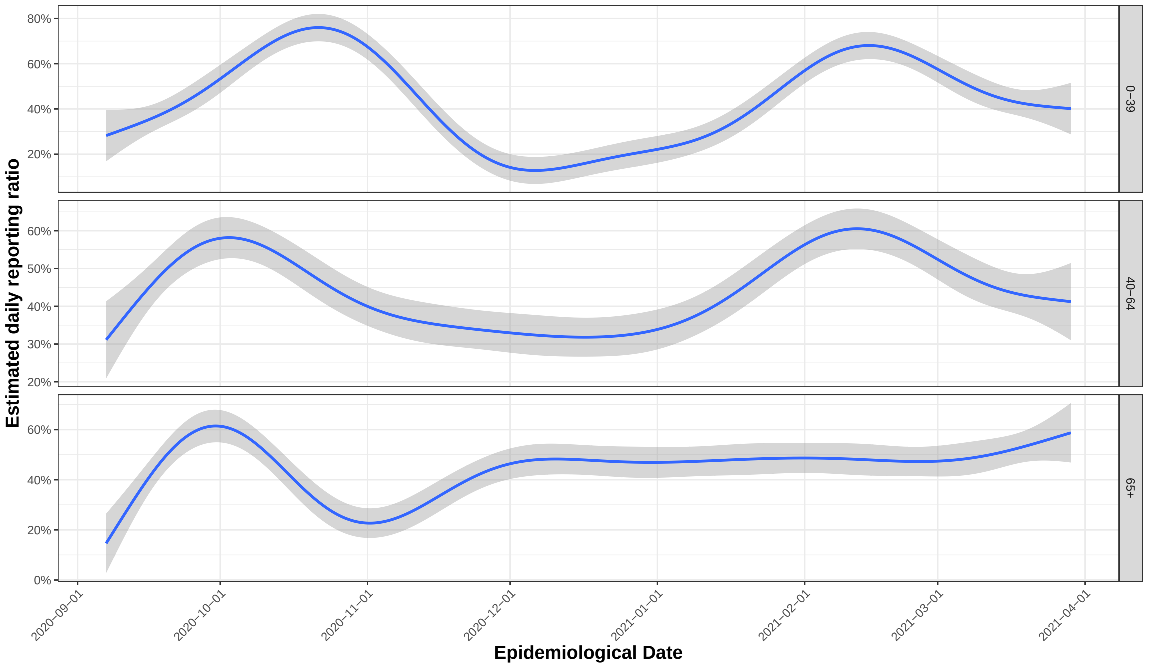


Figure S12: Greece - Estimated age-stratified reporting ratio under the MBM transmission model.

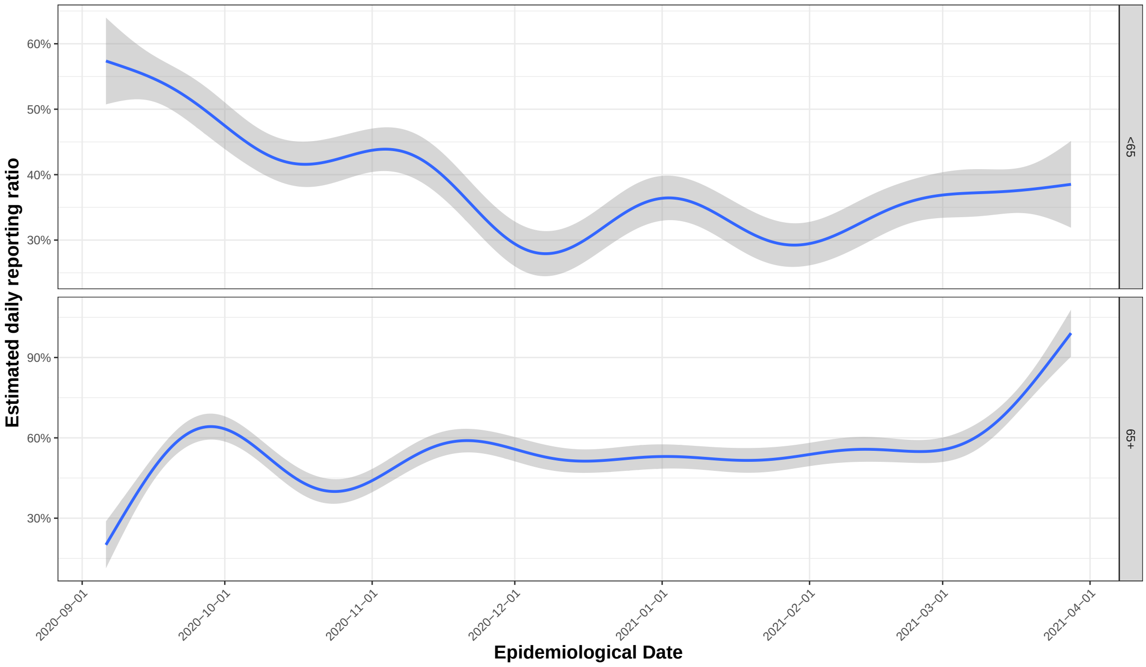


Figure S13: Austria - Estimated age-stratified reporting ratio under the MBM transmission model.
